# Supplementary material for: Style Example-Guided Text Generation using Generative Adversarial Transformers
Source: arXiv:2003.00674 source file (2020-03-02)
Supplement: Supplementary file 1 [file fig_appendix_content_novelty.tex]

\begin{table}[h]
\begin{adjustbox}{width=\columnwidth,center}
    \setlength\extrarowheight{1pt}
    \setlength{\tabcolsep}{2pt}
	\centering
	\begin{tabular}{c || c | c | c | c |}
	    \cline{2-5}
	    & Books vs. News  & Books vs. Reviews & News vs. Reviews & avg. (Upper/Lower Bound))\\ 
	    \hline
	    \multicolumn{1}{|c||}{Cross-Styles}& 35.36 & 34.48 & 30.60 & 33.45\\ \hline
	    \multicolumn{1}{|c||}{Cross-Paragraphs}& 24.94 & 16.94 & 9.34 & 17.07\\ \hline
	\end{tabular}
	\end{adjustbox}
	\caption{Content Novelty by cross styles and cross paragraphs on $3$-styles.}
	\label{tab:appendix_novelty_UB_LB_3}
\end{table}

\begin{table}[h]
\begin{adjustbox}{width=\columnwidth,center}
    \setlength\extrarowheight{1pt}
    \setlength{\tabcolsep}{2pt}
	\centering
	\begin{tabular}{c || c | c | c | c | c | c | c | c | c | c | c | c | c | c | c | c | c | c | c | c | c |}
	    \cline{2-22}
	    & tech news & thriller books  & news & adventure books & life news & sciencefiction books & poetry books &  fantasy books & entertainment news & movie reviews & business news & romance books & lyrics & plays books & sciences news & politic news & opinion news & youndadule books & yelp reviews & hotel reviews & sport news\\ 
	    \hline
	    \multicolumn{1}{|c||}{tech news}& 31.56& 33.06& 32.55& 33.27& 32.5& 33.32& 32.67& 33.6& 32& 29.47& 33.45& 33.55& 29.71& 32.96& 33.02& 33.04& 32.87& 33.67& 29.09& 28.68& 33.33\\ \hline
	    \multicolumn{1}{|c||}{thriller books}& 32.78& 28.4& 32.84& 28.56& 32.67& 28.77& 29.61& 28.38& 32.65& 30.31& 33.89& 28.81& 29.86& 29.53& 33.41& 32.49& 33.2& 28.38& 29.77& 29.57& 33.35\\ \hline
	    \multicolumn{1}{|c||}{news}& 32.56& 33.28& 33.27& 33.28& 33.45& 32.97& 32.84& 33.71& 33& 30.72& 33.08& 33.73& 30.78& 33.22& 33.21& 32.98& 33.23& 33.77& 30.07& 29.58& 33.79\\ \hline
	    \multicolumn{1}{|c||}{adventure books}& 33.54& 28.53& 32.95& 28.67& 33.13& 28.28& 29.94& 29.2& 32.87& 31.14& 34.04& 28.89& 30.51& 29.66& 32.95& 33.6& 34.43& 28.33& 31.05& 30.66& 33.77\\ \hline
	    \multicolumn{1}{|c||}{life news}& 32.85& 32.89& 33.26& 33.16& 33.02& 33.23& 32.76& 33.47& 33.4& 31.19& 34.03& 33.46& 31& 33.03& 33.37& 33.48& 34.1& 33.42& 30.84& 30.55& 33.97\\ \hline
	    \multicolumn{1}{|c||}{sciencefiction books}& 33.38& 28.41& 33.21& 28.14& 33.04& 28.8& 29.91& 28.57& 32.54& 30.59& 33.87& 28.38& 30.19& 29.77& 33.04& 33.2& 33.87& 28.18& 30.17& 30.09& 33.06\\ \hline
	    \multicolumn{1}{|c||}{poetry books}& 32.85& 30.31& 32.72& 30.26& 32.24& 30.53& 29.18& 30.1& 32.81& 30.42& 33.38& 30.81& 29.9& 29.5& 32.79& 33.35& 34.06& 30.14& 30.42& 30.23& 33.46\\ \hline
	    \multicolumn{1}{|c||}{fantasy books}& 33.58& 28.6& 33.59& 28.54& 32.76& 28.45& 29.89& 28.33& 33.23& 31.3& 34.47& 28.93& 31.05& 29.97& 33.49& 33.62& 34.15& 28.6& 31.25& 31.16& 34.06\\ \hline
	    \multicolumn{1}{|c||}{entertainment news}& 32.37& 33.05& 32.16& 32.99& 32.8& 32.85& 32.34& 32.94& 31.87& 28.59& 33.44& 33.14& 29.37& 32.13& 33.16& 33.8& 33.43& 33.19& 28.57& 28.26& 33.28\\ \hline
	    \multicolumn{1}{|c||}{movie reviews}& 29.78& 31.15& 30.35& 31.19& 30.61& 31& 30.04& 31.32& 29.36& 18.53& 31.81& 31.39& 24.31& 30.23& 31.77& 31.13& 30.44& 31.21& 20.54& 18.91& 31.26\\ \hline
	    \multicolumn{1}{|c||}{business news}& 33.33& 33.9& 34.03& 34.04& 33.29& 34.08& 33.65& 33.89& 33.93& 32.15& 33.42& 34.41& 32.5& 33.8& 33.49& 33.03& 34.12& 34.44& 31.76& 31.53& 34.06\\ \hline
	    \multicolumn{1}{|c||}{romance books}& 33.87& 28.31& 33.69& 28.46& 33.57& 28.86& 30.29& 29.07& 33.14& 31.52& 34.51& 28.89& 31.35& 30.08& 33.85& 33.29& 34.47& 28.69& 30.94& 30.96& 34.08\\ \hline
	    \multicolumn{1}{|c||}{lyrics}& 29.87& 30.73& 30.32& 30.47& 30.78& 30.46& 29.17& 30.45& 29.47& 23.78& 31.76& 30.76& 21.83& 29.54& 32.27& 31.17& 30.68& 30.78& 23.38& 21.84& 31.52\\ \hline
	    \multicolumn{1}{|c||}{plays books}& 32.88& 29.95& 32.7& 29.64& 32.23& 29.69& 29.63& 30.22& 32.27& 30.05& 33.78& 30.37& 29.94& 29.31& 33.03& 33.12& 33.68& 29.56& 30.05& 29.61& 33.57\\ \hline
	    \multicolumn{1}{|c||}{sciences news}& 32.81& 33.42& 32.85& 33.33& 32.88& 33.24& 32.06& 33.56& 33.18& 30.84& 33.35& 33.79& 31.22& 32.82& 32.96& 33.2& 33.49& 33.35& 30.54& 30.15& 33.91\\ \hline
	    \multicolumn{1}{|c||}{politic news}& 32.51& 33.44& 32.72& 33.47& 32.69& 33.2& 32.9& 33.7& 32.72& 31.1& 32.72& 33.62& 31.08& 33.11& 33.26& 32.31& 33.49& 32.99& 30.74& 30.17& 33.27\\ \hline
	    \multicolumn{1}{|c||}{opinion news}& 33.23& 33.68& 33.4& 33.75& 33.19& 33.69& 33.32& 33.52& 33.82& 31.35& 33.86& 34.05& 31.88& 33.41& 33.54& 33.98& 33.92& 34.43& 31.41& 30.96& 34.11\\ \hline
	    \multicolumn{1}{|c||}{youndadule books}& 33.91& 28.06& 33.74& 28.75& 33.78& 28.47& 30.27& 28.48& 33.47& 31.4& 34.48& 28.57& 31.22& 29.61& 33.65& 34.07& 34.57& 28.68& 31.13& 31.03& 33.82\\ \hline
	    \multicolumn{1}{|c||}{yelp reviews}& 29.39& 31.16& 30.34& 31.19& 30.81& 30.97& 30.22& 31.3& 30.34& 21.03& 31.75& 31.28& 24.27& 30.36& 32.16& 31.16& 30.63& 31.2& 18.88& 17.62& 31.44\\ \hline
	    \multicolumn{1}{|c||}{hotel reviews}& 28.66& 31.05& 29.51& 30.99& 30.06& 30.95& 29.99& 31.16& 29.13& 18.58& 31.23& 31.19& 22.14& 30& 31.5& 30.7& 29.65& 31.08& 16.78& 13.33& 30.64\\ \hline
	    \multicolumn{1}{|c||}{sport news}& 34.09& 34.45& 34.74& 34.01& 33.85& 34.24& 33.24& 34.19& 34.08& 31.46& 35.31& 34.77& 32.34& 33.91& 34.84& 34.3& 34.97& 34.1& 31.9& 31.26& 34.25\\ \hline
	\end{tabular}
	\end{adjustbox}
	\caption{Content Novelty by cross styles on $21$-styles.}
	\label{tab:appendix_novelty_UB_21}
\end{table}
\begin{table}[h]
\begin{adjustbox}{width=\columnwidth,center}
    \setlength\extrarowheight{1pt}
    \setlength{\tabcolsep}{2pt}
	\centering
	\begin{tabular}{c || c | c | c | c | c | c | c | c | c | c | c | c | c | c | c | c | c | c | c | c | c |}
	    \cline{2-22}
	    & tech news & thriller books  & news & adventure books & life news & sciencefiction books & poetry books &  fantasy books & entertainment news & movie reviews & business news & romance books & lyrics & plays books & sciences news & politic news & opinion news & youndadule books & yelp reviews & hotel reviews & sport news\\ 
	    \hline
	    \multicolumn{1}{|c||}{Style Diversity}& 15.91&  16.72&  16.29& 17.33& 17.73& 16.77& 14.37& 15.82& 15.62& 9.00& 17.46& 15.63& 11.88& 15.56& 17.16& 17.20&  16.95& 15.58& 9.00& 8.15& 17.59\\ \hline
	\end{tabular}
	\end{adjustbox}
	\caption{Content Novelty by cross paragraphs on $21$-styles.}
	\label{tab:appendix_novelty_LB_21}
\end{table}
