# Supplementary material for: Style Example-Guided Text Generation using Generative Adversarial Transformers
Source: arXiv:2003.00674 source file (2020-03-02)
Supplement: Supplementary file 2 [file fig_appendix_key_terms.tex]

{\bf Sciences News:} \textit{science, environment, sea-levels, space.com, planet,	panda, species, climate-change,	/science/,	-science-, scientist,	scientism,	/future/,	/earth/,	global-warming,	spaceflight,	magellan}

{\bf Sport News:} \textit{epsn,	football,	baseball,	basketball,	49ers,	ftw, -sport-,	/sport/,	-sports-,	/sports/,	-nfl-,	/nfl/,	athlete,	thepostgame,	golf,	soccer,	ncaa,	volleyball,	/nba/,	-nba-,	/mlb/,	-mlb-,	super-bowl}

{\bf Politic News:} \textit{democrats,	republicans,	trump,	congress,	politic,	clinton,	hillary,	defense,	clarification,	president,	military,	hotair,	antiwar,	capitalism,	council,	election,	senator,	obama,	senate,	government,	isis,	russia}

{\bf Business News:} \textit{forbes,	money,	business,	econom,	wsj,	economist,	fool.com,	companies,	cityam.com,	entrepreneurship,	vccircle.com,	bloomberg.com,	accenture,	pionline.com,	bank,	crainsdetroit,	seekingalpha,	domainnamewire,	xconomy,	dealbreaker,	gallup.com,	kickstarter}

{\bf Technology News:} \textit{geekwire,	cyber,	tech,	macbook,	facebook,	twitter,	google,	mobile,	android, website,	live-stream,	gigaom,	venturebeat, ipod,	gizmodo,	cnet,	thenextweb,	digitaltrends,	in.pcmag.com,	zdnet,	geek.com, /auto/,	-auto-,	/cars/,	/car/,	automation,	apps,	/autos/,	-autos-,	iphone,	samsung,	instagram,	oculus,	hololens,	360-video,	hyperloop,	amazon,	lenovo,	steve-jobs,	tim-cook,	microsoft,	surveillance-system,	outlook,	htc,	nintendo,	3d-print, ipad,	apple-pay,	skylanders,	vivofit,	viber,	apple-watch,	motorola,	silicon-valley,	bitcoin,	-ipo,	mozilla	,self-driving,	apple-app,	tesla,	toshiba,	myspace,	vizio,	nokia,	panasonic,	startup,	fitbit,	whatsapp,	icloud,	zuckerberg,	qardio, alibaba,	intel-,	imac,	snapchat,	acer,	linkedin,	airpods,	playstation,	smartphone}

{\bf Entertainment News:} \textit{celebrity,	fashion,	entertain,	music,	movie,	film,	lithgow,	stage,	selfie,	collider.com,	hiphopwired,	olivia-newton,	hollywood,	screenrant,	digitalspy,	kotaku,	/tv/,	-tv-,	/tvs/,	-tvs-,	deadline.com,	thewrap.com,	tasteofcountry,	theboombox,	/style/, /royals/,	/awards/,	http://people.com/country/,	https://www.hellomagazine.com/,	artanddesign,	madonna}

{\bf Opinion News:} \textit{/blog/,	comment, opinion,	/story/,	theobserver,	education, subscription, bully, salon.com,	thedailybeast,	sheknows,	magazine,  theatlantic.com/family/,	yourtango,	/stories/,	/culture/}

{\bf Life News:} \textit{rheumatoid,	travel,	lifestyle,	living,	life-style,	leisure,	/home/,	castle,	lifeandstyle, cities,	washingtonian,	rural-life, jewcy,	wwd,	mashable,	product-reviews.net,	-ad-,	advertisement,	health,	/home/,	/babies/,	/parents/,	/food/, /pets/,	/bodies/,	greatideas.people.com}

{\bf News News:} \textit{world,	uk,	german,	london,	theborneopost,	allafrica,	philippine,	pemex,	japan,	iceland,	kwacha,	israel,	macleans.ca, new-york,	national,	us,	nypost,	media,	video,	news,	org,	crime,	transcript,	society,	weather,	latino,	latimes,	ny,	express,	boston,	rafu,	california,	huffpost,	chicago,	wtkr,	csmonitor,	u-s,
kfor,	cbslocal,	chrisd.ca,	marinij,	orlando,	oregon,	pe.com,	newyork,	minnpost,	myfox8,	cornellsun,	ktla,	theday,	santacruz,	camp-fire,	kdvr.com,	denverpost,	lehighvalleylive,	redlandsdailyfacts,	kcci,	wmur,	kcra,	fox13now,	wgnradio,
montereyherald,	ocregister,	fox59,	washington,	/crime/}

\begin{table}[h]
\begin{adjustbox}{width=\columnwidth,center}
    \setlength\extrarowheight{1pt}
    \setlength{\tabcolsep}{2pt}
	\centering
	\begin{tabular}{c || c | c | c | c | c | c | c | c | c |}
	    \cline{2-10}
	    & tech news & news & life news & entertainment news & business news & sciences news & politic news & opinion news & sport news\\ 
	    \hline
	    \multicolumn{1}{|c||}{\# documents}& 2.7M & 12M & 1.2M & 2.9M & 2.6M & 0.3M & 2.7M & 1.7M & 2.7M \\ \hline
	\end{tabular}
	\end{adjustbox}
	\caption{Number of documents in the style-RealNews dataset.}
	\label{tab:appendix_style_realnews}
\end{table}
