# Supplementary material for: Style Example-Guided Text Generation using Generative Adversarial Transformers
Source: arXiv:2003.00674 source file (2020-03-02)
Supplement: Supplementary file 3 [file fig_appendix_style_diversity.tex]

% \begin{table}[h]
% \begin{adjustbox}{width=\columnwidth,center}
%     \setlength\extrarowheight{1pt}
%     \setlength{\tabcolsep}{2pt}
% 	\centering
% 	\begin{tabular}{c || c | c | c | c |}
% 	    \cline{2-5}
% 	    & Books vs. News  & Books vs. Reviews & News vs. Reviews & avg. (Upper/Lower Bound))\\ 
% 	    \hline
% 	    \multicolumn{1}{|c||}{Cross-Styles}& 15.56 & 14.75 & 15.92 & 15.41\\ \hline
% 	    \multicolumn{1}{|c||}{Cross-Paragraphs}& 7.44 & 4.79 & 4.75 & 5.66\\ \hline
% 	\end{tabular}
% 	\end{adjustbox}
% 	\caption{Style Diversity by cross styles and cross paragraphs on $3$-styles.}
% 	\label{tab:appendix_diversity_UB_LB_3}
% \end{table}

\begin{table}[!t]
\begin{adjustbox}{width=\columnwidth,center}
    \setlength\extrarowheight{1pt}
    \setlength{\tabcolsep}{2pt}
	\centering
	\begin{tabular}{c || c | c | c | c | c | c | c | c | c | c | c | c | c | c | c | c | c | c | c | c | c |}
	    \cline{2-22}
	    & tech news & thriller books  & news & adventure books & life news & sciencefiction books & poetry books &  fantasy books & entertainment news & movie reviews & business news & romance books & lyrics & plays books & sciences news & politic news & opinion news & youndadule books & yelp reviews & hotel reviews & sport news\\ 
	    \hline
	    \multicolumn{1}{|c||}{tech news}& 14.8&  15.4&  15.66& 15.52& 15.38& 15.43& 16.15& 15.92& 15.22& 15.54& 15.27& 16.03& 17.16& 15.96& 15.18& 15.6&  16.13& 15.81& 16.44& 16.69& 16.44\\ \hline
	    \multicolumn{1}{|c||}{thriller books}& 15.41& 9.43&  14.97& 9.64&  14.56& 9.6&   12.51& 10.17& 14.03& 13.77& 15.73& 9.83&  13.62& 12.17& 14.91& 15.09& 16.13& 9.7&   14.63& 15.1&  15.44\\ \hline
	    \multicolumn{1}{|c||}{news}& 15.67& 14.94& 15.32& 15.1&  15.3&  15.05& 15.88& 15.48& 15.19& 15.5&  15.49& 15.56& 16.99& 15.71& 15.19& 15.13& 16.13& 15.36& 16.55& 16.74& 16.09\\ \hline
	    \multicolumn{1}{|c||}{adventure books}& 15.58& 9.71&  15.14& 9.63&  14.73& 9.67&  12.51& 10.07& 14.19& 13.89& 15.9&  9.88&  13.62& 12.2&  15.04& 15.23& 16.29& 9.67&  14.78& 15.23& 15.59\\ \hline
	    \multicolumn{1}{|c||}{life news}& 15.45& 14.56& 15.31& 14.7&  14.84& 14.62& 15.36& 15.07& 14.82& 15.09& 15.54& 15.13& 16.38& 15.29& 14.96& 15.33& 16.14& 14.91& 15.82& 16.21& 16.11\\ \hline
	    \multicolumn{1}{|c||}{sciencefiction books}& 15.43& 9.6&   15.02& 9.55&  14.66& 9.41&  12.32& 9.83&  14.14& 13.79& 15.78& 9.74&  13.51& 12.11& 14.9&  15.12& 16.17& 9.52&  14.77& 15.27& 15.49\\ \hline
	    \multicolumn{1}{|c||}{poetry books}& 16.13& 12.49& 15.84& 12.39& 15.41& 12.25& 11.8&  12.3&  15.04& 14.48& 16.41& 12.65& 12.61& 12.72& 15.52& 16.01& 16.69& 12.45& 15.44& 15.87& 16.43\\ \hline
	    \multicolumn{1}{|c||}{fantasy books}& 15.87& 10.1&  15.4&  9.94&  15.04& 9.72&  12.32& 9.75&  14.56& 14.23& 16.18& 10.09& 13.58& 12.29& 15.27& 15.54& 16.51& 9.7&   15.21& 15.68& 15.88\\ \hline
	    \multicolumn{1}{|c||}{entertainment news}& 15.28& 14.05& 15.16& 14.23& 14.82& 14.17& 15.07& 14.62& 13.6&  14.21& 15.69& 14.58& 15.87& 14.71& 15.13& 15.29& 16.07& 14.41& 15.73& 16.3&  15.7\\ \hline
	    \multicolumn{1}{|c||}{movie reviews}& 15.42& 13.7&  15.39& 13.79& 14.99& 13.75& 14.42& 14.2&  14.09& 11.28& 15.91& 14.21& 15.3&  13.98& 15.07& 15.44& 16.26& 14.03& 14.29& 14.96& 15.92\\ \hline
	    \multicolumn{1}{|c||}{business news}& 15.42& 15.78& 15.54& 15.98& 15.56& 15.88& 16.49& 16.33& 15.74& 16.01& 14.58& 16.44& 17.63& 16.39& 15.16& 15.34& 15.95& 16.24& 16.84& 17.04& 16.56\\ \hline
	    \multicolumn{1}{|c||}{romance books}& 16.05& 9.89&  15.58& 9.93&  15.15& 9.82&  12.71& 10.23& 14.57& 14.33& 16.39& 9.72&  13.76& 12.44& 15.55& 15.72& 16.73& 9.71&  15.09& 15.58& 15.97\\ \hline
	    \multicolumn{1}{|c||}{lyrics}& 17.16& 13.59& 16.96& 13.58& 16.37& 13.56& 12.7&  13.61& 15.91& 15.35& 17.57& 13.7&  11.46& 13.3&  16.78& 17.15& 17.87& 13.71& 16.01& 16.44& 17.29\\ \hline
	    \multicolumn{1}{|c||}{plays books}& 16.05& 12.16& 15.82& 12.21& 15.34& 12.13& 12.78& 12.22& 14.84& 14.1&  16.41& 12.37& 13.35& 11.87& 15.66& 16& 16.66& 12.26& 15& 15.47& 16.28\\ \hline
	    \multicolumn{1}{|c||}{sciences news}& 15.28& 14.9&  15.13& 14.99& 14.92& 14.92& 15.55& 15.34& 15.04& 15.18& 15.03& 15.54& 16.77& 15.64& 14.02& 14.92& 15.75& 15.27& 16.36& 16.65& 16.19\\ \hline
	    \multicolumn{1}{|c||}{politic news}& 15.54& 14.99& 15.06& 15.11& 15.22& 15.09& 15.9&  15.54& 15.21& 15.48& 15.22& 15.64& 17.09& 15.85& 14.87& 14.33& 15.99& 15.46& 16.76& 16.95& 16.19\\ \hline
	    \multicolumn{1}{|c||}{opinion news}& 16.22& 16.14& 16.21& 16.28& 16.09& 16.19& 16.76& 16.61& 16.12& 16.4&  15.96& 16.7&  17.82& 16.61& 15.93& 16.16& 16.49& 16.54& 17.33& 17.59& 17.13\\ \hline
	    \multicolumn{1}{|c||}{youndadule books}& 15.78& 9.64&  15.35& 9.58&  14.88& 9.49&  12.51& 9.83&  14.34& 14.06& 16.1&  9.62&  13.67& 12.21& 15.21& 15.46& 16.48& 9.38&  14.9&  15.44& 15.75\\ \hline
	    \multicolumn{1}{|c||}{yelp reviews}& 16.32& 14.58& 16.44& 14.69& 15.75& 14.69& 15.43& 15.2&  15.62& 14.27& 16.74& 14.98& 15.97& 14.92& 16.29& 16.7&  17.22& 14.88& 11.59& 12.97& 16.83\\ \hline
	    \multicolumn{1}{|c||}{hotel reviews}& 16.66& 15.1&  16.69& 15.21& 16.18& 15.27& 15.88& 15.72& 16.25& 14.95& 16.99& 15.53& 16.44& 15.44& 16.58& 16.98& 17.56& 15.48& 12.9&  10.93& 17.27\\ \hline
	    \multicolumn{1}{|c||}{sport news}& 16.41& 15.41& 16.09& 15.51& 16.03& 15.49& 16.44& 15.89& 15.67& 15.96& 16.48& 15.92& 17.27& 16.14& 16.17& 16.13& 17.09& 15.74& 16.87& 17.27& 15.21\\ \hline
	\end{tabular}
	\end{adjustbox}
	\caption{Upper bounds of the style diversity measured using the $21$-style dataset.}
	\label{tab:appendix_diversity_UB_21}
\end{table}

\begin{table}[!t]
\begin{adjustbox}{width=\columnwidth,center}
    \setlength\extrarowheight{1pt}
    \setlength{\tabcolsep}{2pt}
	\centering
	\begin{tabular}{c || c | c | c | c | c | c | c | c | c | c | c | c | c | c | c | c | c | c | c | c | c |}
	    \cline{2-22}
	    & tech news & thriller books  & news & adventure books & life news & sciencefiction books & poetry books &  fantasy books & entertainment news & movie reviews & business news & romance books & lyrics & plays books & sciences news & politic news & opinion news & youndadule books & yelp reviews & hotel reviews & sport news\\ 
	    \hline
	    \multicolumn{1}{|c||}{Style Diversity}& 4.82&  4.18&  4.68& 4.12& 4.67& 4.04& 4.02& 4.01& 4.8& 4.78& 4.77& 3.99& 4.37& 4.53& 4.6& 4.73&  4.98& 3.95& 4.8& 5.38& 4.71\\ \hline
	\end{tabular}
	\end{adjustbox}
	\caption{Lower bounds of the style diversity measured using the $21$-style dataset.}
	\label{tab:appendix_diversity_LB_21}
\end{table}
