# Supplementary material for: Style Example-Guided Text Generation using Generative Adversarial Transformers
Source: arXiv:2003.00674 source file (2020-03-02)
Supplement: Supplementary file 4 [file fig_appendix_ablation_study.tex]

\begin{table}[h]
    \setlength\extrarowheight{1pt}
    \setlength{\tabcolsep}{1pt}
	\centering
	\begin{tabular}{| c || c | c | c | c |}
	    \cline{1-5}
	    Model D & Fluency Score  &  Style Score  & Style Diversity & Content Novelty \\ 
	    \hline
	    \multicolumn{1}{|c||}{w/o $\mathcal{L}_{DIST}$}& 7.13 & 90.46 & 10.11 & 26.95\\ \hline
	    \multicolumn{1}{|c||}{w/o $\mathcal{L}_{STYLE}$} & 4.52 & 34.87 & 15.27 & 28.00\\ \hline
	    \multicolumn{1}{|c||}{ w/o $\mathcal{L}_{GAN}$} & 7.25 & 72.5 & 10.71 & 31.69 \\ \hline
	    \multicolumn{1}{|c||}{All} & 7.18 & 70.94 & 11.13 & 28.00 \\ \hline
	\end{tabular}
	\caption{Ablation Study on $3$-styles.}
	\label{tab:ablation_study_3}
\end{table}
