# Supplementary material for: Style Example-Guided Text Generation using Generative Adversarial Transformers
Source: arXiv:2003.00674 source file (2020-03-02)
Supplement: Supplementary file 5 [file fig_appendix_dialogue_books.tex]

\begin{table}[h]
\begin{adjustbox}{width=\columnwidth,center}
    \setlength\extrarowheight{1pt}
    \setlength{\tabcolsep}{2pt}
	\centering
	\begin{tabular}{c || c | c | c | c | c | c | c | c |}
	    \cline{2-9}
	    & Romance & Fantasy & Sciencefiction & Youngadultorteen/Children’sbooks/Educational & Thriller/suspense/Mystery/detective & Adventure & Poetry (non-dialogue) & Plays (non-dialogue)\\ 
	    \hline
	    \multicolumn{1}{|c||}{\# documents}& 160K & 148K & 112K & 122K & 114K & 34K & 79K & 28K\\ \hline
	\end{tabular}
	\end{adjustbox}
	\caption{Number of documents in the Dialogue-BookCorpus dataset.}
	\label{tab:appendix_dialogue_books}
\end{table}
