# Supplementary material for: Style Example-Guided Text Generation using Generative Adversarial Transformers
Source: arXiv:2003.00674 source file (2020-03-02)
Supplement: Supplementary file 6 [file fig_appendix_fluency_vs_style.tex]

\begin{figure}[h]
\begin{subfigure}{.5\textwidth}
  \centering
  \includegraphics[width=\linewidth]{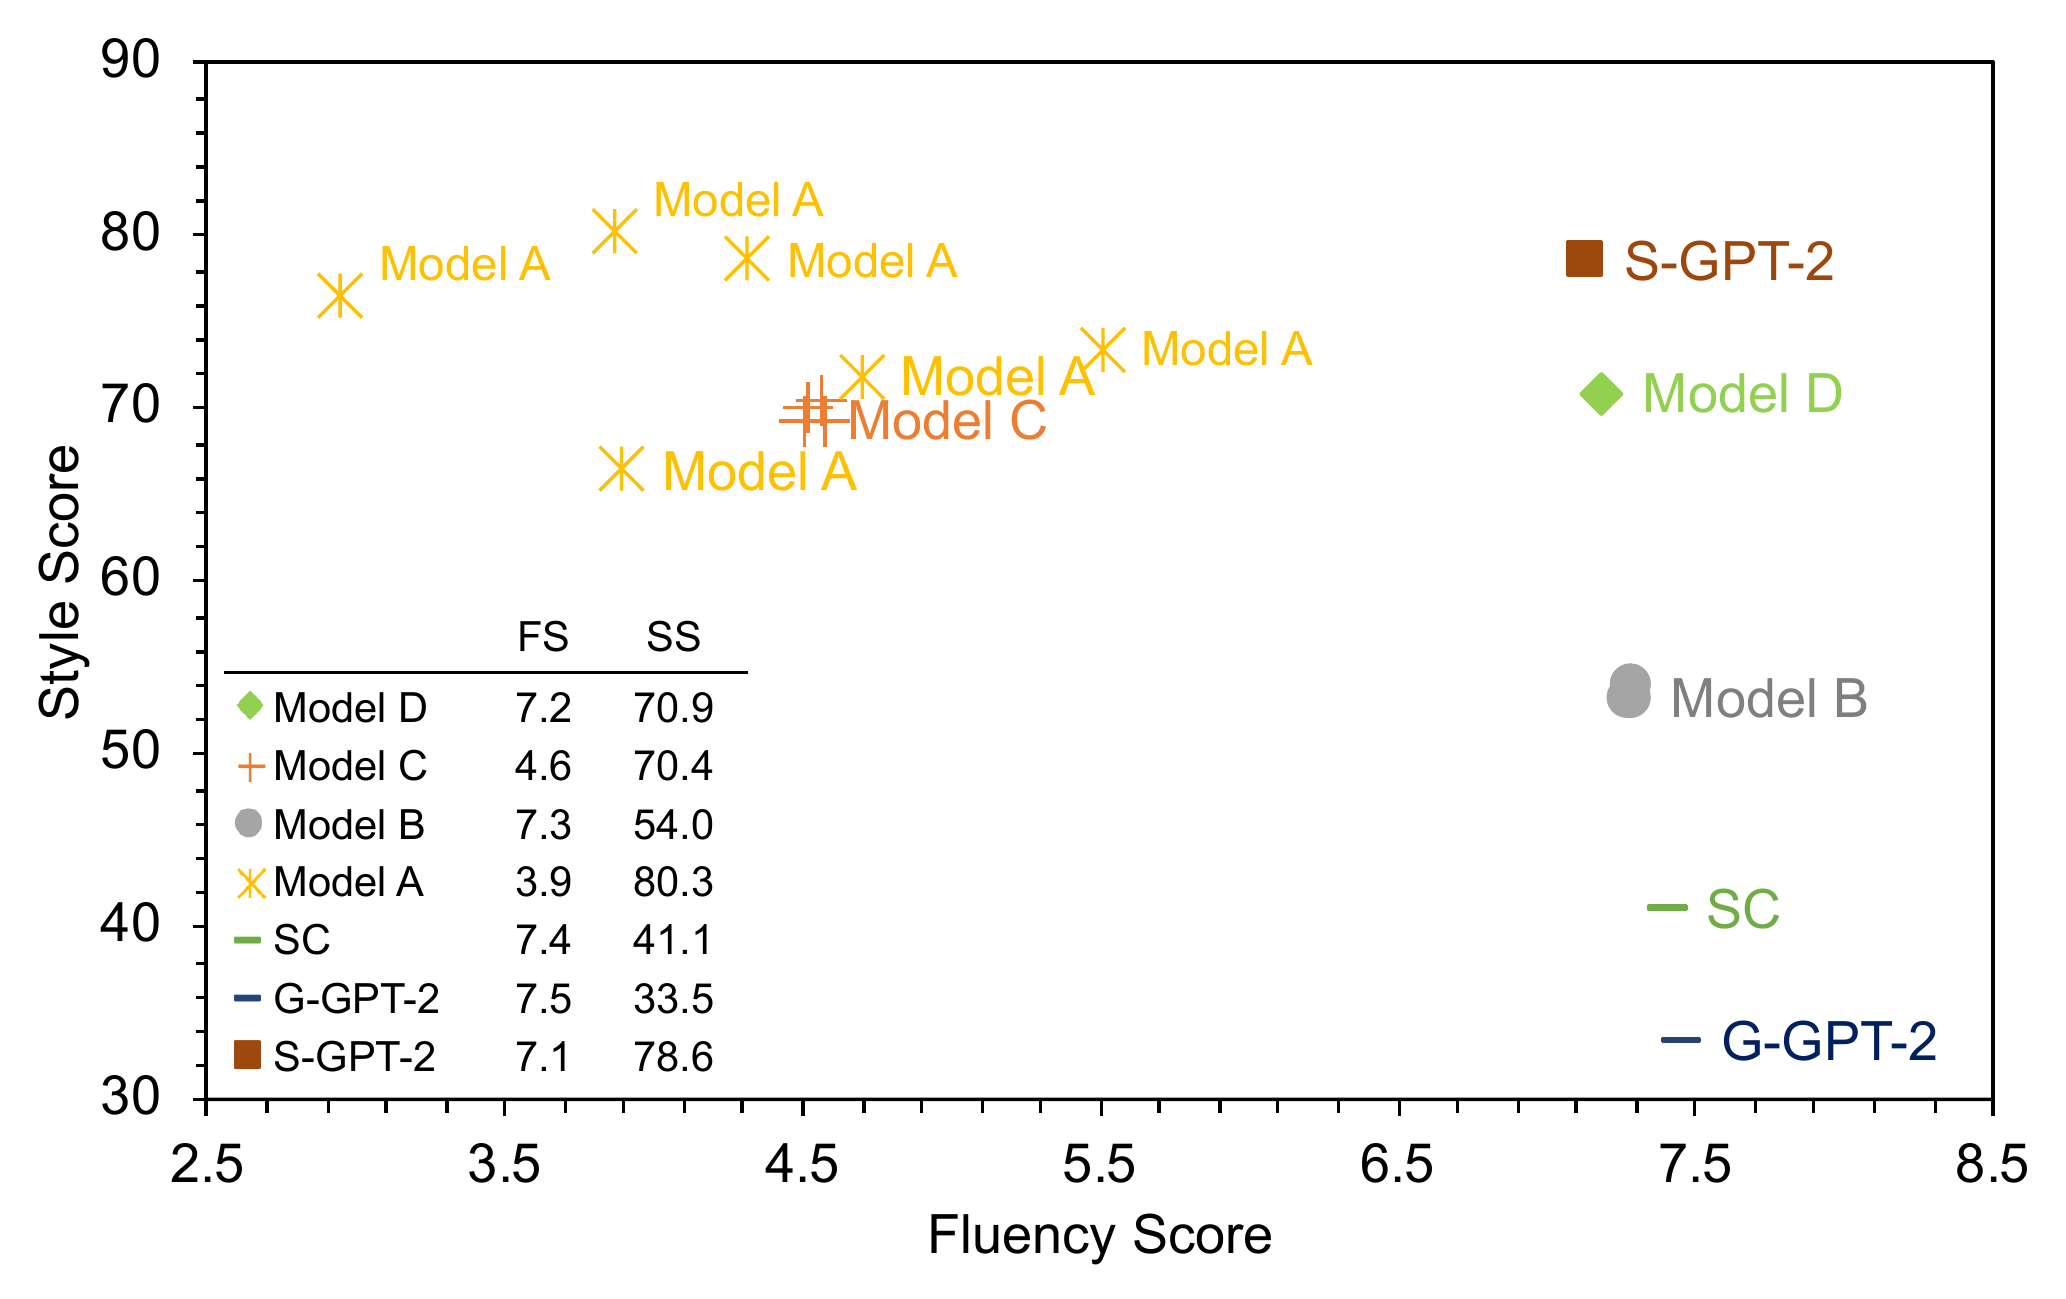}
  \caption{Fluency score vs. style score on 3 styles.}
  \label{fig:sfig1}
\end{subfigure}%
\begin{subfigure}{.5\textwidth}
  \centering
  \includegraphics[width=\linewidth]{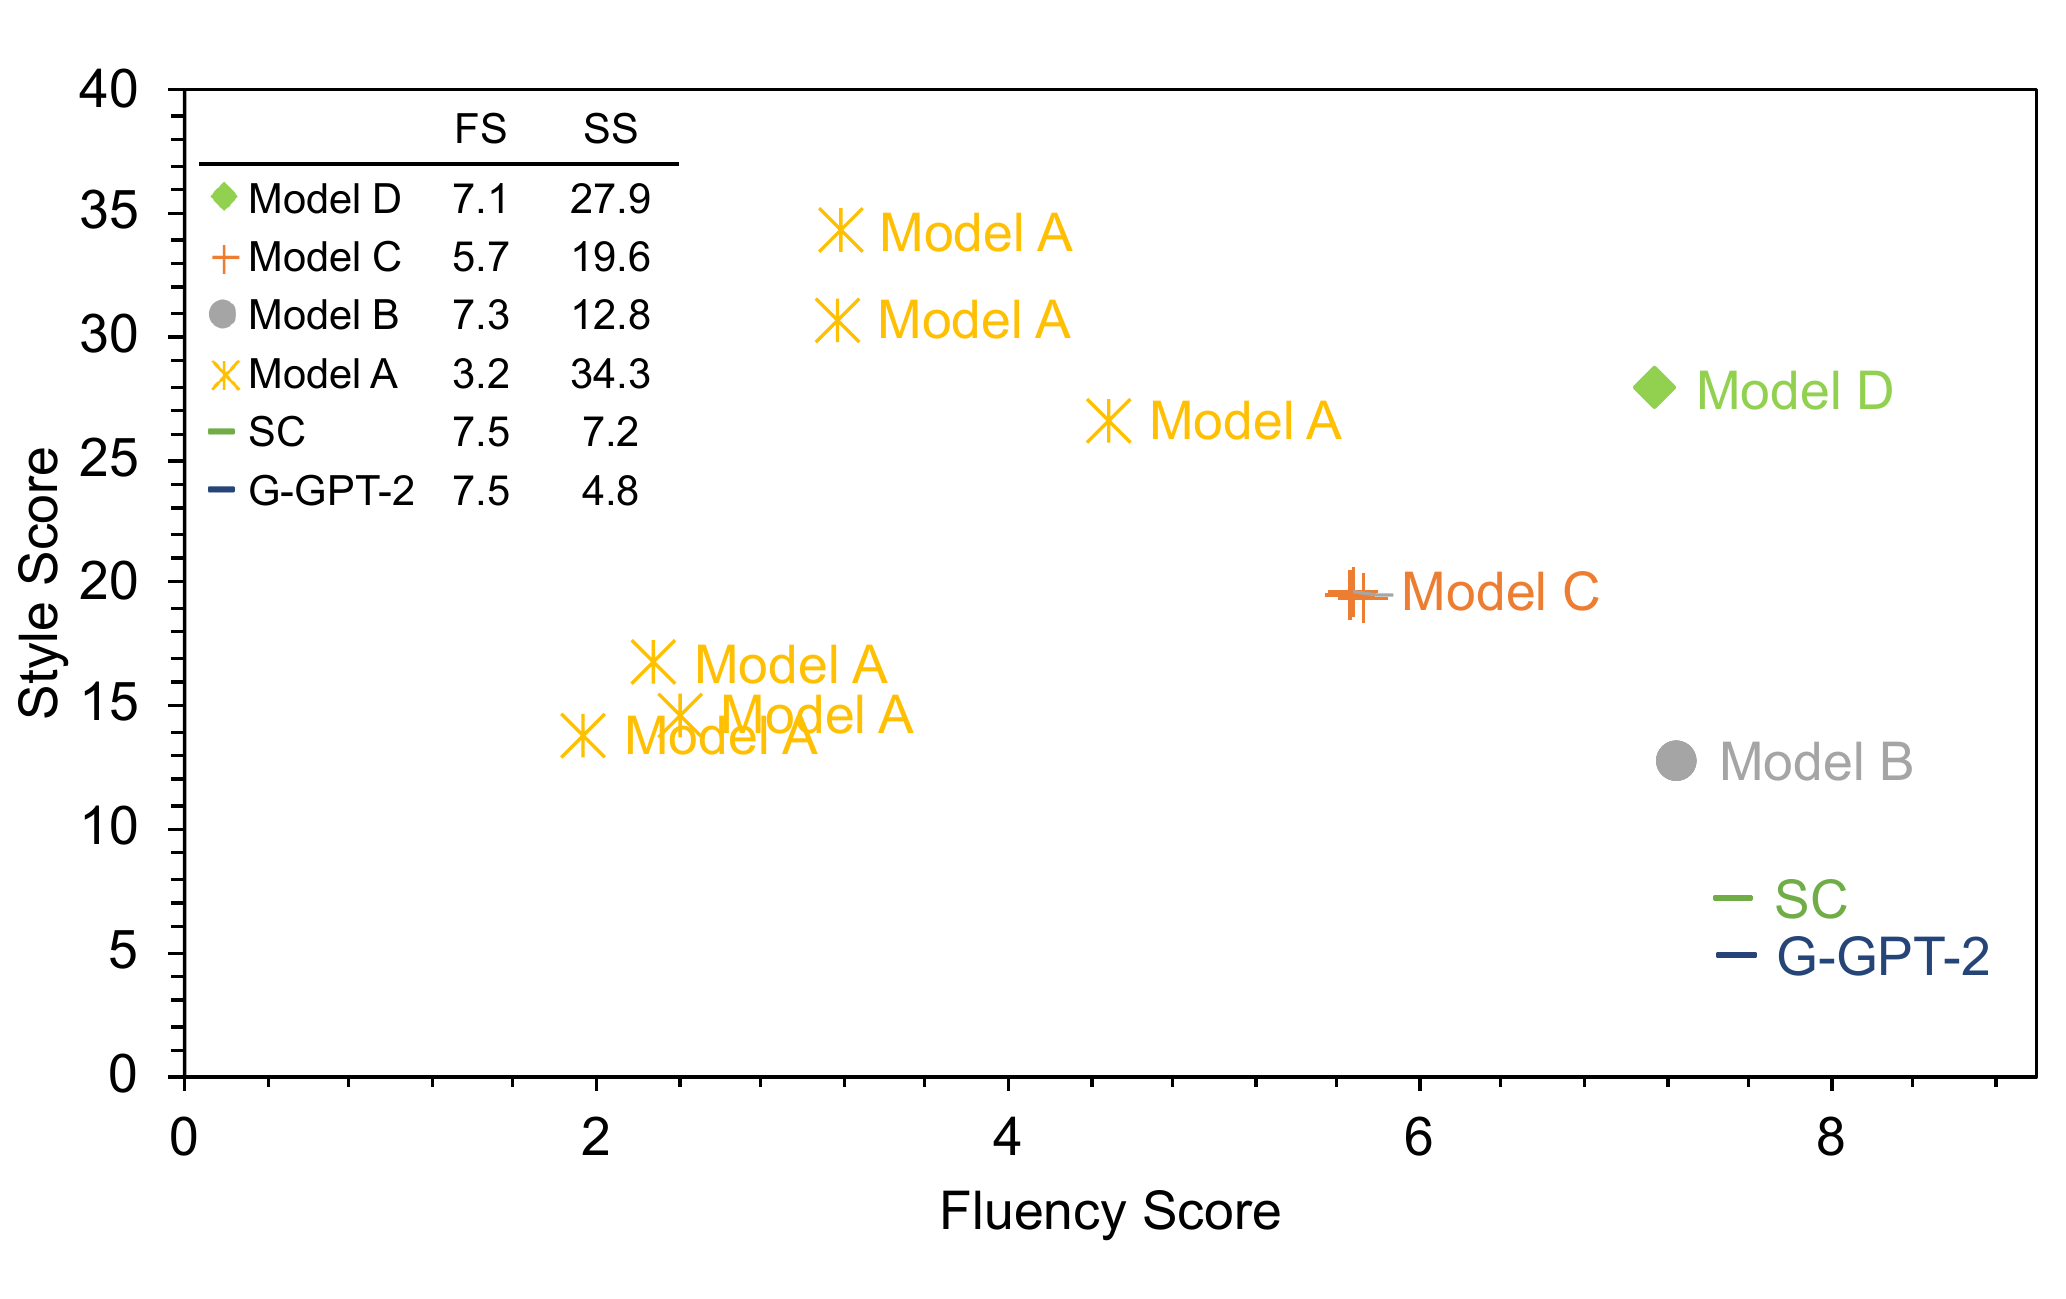}
  \caption{Fluency score vs. style score on 21 styles.}
  \label{fig:sfig2}
\end{subfigure}
\caption{Fluency score vs. style score results on both 3 styles and 21 styles datasets. \textit{G-GPT-2} denotes general GPT-2, \textit{S-GPT-2} denotes specialize GPT-2, \textit{SC} denotes Style-Code Encoding baseline. \textit{Model A, B, C, D} are our proposed models.}
\label{fig:fluency_vs_style_all}
\end{figure}
